# Supplementary material for: Angelic Processes
Source: arXiv:1505.04726 source file (2015-05-28)
Supplement: Supplementary file 2 [file appendix-designs-pbmh-links.tex]

\chapter{Linking theories}\label{appendix:links}

\section{$acdash2ac$ and $ac2acdash$}

\begin{law}[$acdash2ac$-subset]\label{law:acdash2ac-subset}
\begin{align*}
	&acdash2ac (t) \subseteq acdash2ac (z) \iff t \subseteq z
\end{align*}
\begin{proof} To be established. \end{proof}
\end{law}

\begin{law}[$ac2acdash$-subset]\label{law:ac2acdash-subset}
\begin{align*}
	&ac2acdash (t) \subseteq ac2acdash (z) \iff t \subseteq z
\end{align*}
\begin{proof} To be established. \end{proof}
\end{law}

\begin{law}[$acdash2ac$-$\emptyset$]\label{law:acdash2ac:emptyset}
\begin{align*}
	&acdash2ac(\emptyset) = \emptyset&
\end{align*}
\begin{proof}
\begin{flalign*}
	&acdash2ac(\emptyset)
	&&\ptext{Definition of $acdash2ac$}\\
	&=\left\{\begin{array}{l} 
			z_0 : S_{in\alpha P}, z_1 : S_{out\alpha P} \\
			| z_0 \in \emptyset \land (\bigwedge x : \alpha P \spot z_0.x = z_1.(x')) \spot z_1 
			\end{array}\right\}
	&&\ptext{Property of sets}\\
	&=\{ z_0 : S_{in\alpha P}, z_1 : S_{out\alpha P} | false \}
	&&\ptext{Property of sets}\\
	&=\emptyset
%	&acdash2ac(t) \subseteq \emptyset
%	&&\ptext{Definition of $acdash2ac$}\\
%	&\iff \left\{\begin{array}{l} 
%			z_0 : S_{in\alpha P}, z_1 : S_{out\alpha P} \\
%			| z_0 \in t \land (\bigwedge x : \alpha P \spot z_0.x = z_1.(x')) \spot z_1 
%			\end{array}\right\} = \emptyset
%	&&\ptext{Property of sets}\\
%	&\iff \forall z \spot z \notin \left\{\begin{array}{l} 
%			z_0 : S_{in\alpha P}, z_1 : S_{out\alpha P} \\
%			| z_0 \in t \land (\bigwedge x : \alpha P \spot z_0.x = z_1.(x')) \spot z_1 
%			\end{array}\right\}
%	&&\ptext{Property of sets}\\
%	&\iff \forall z \spot \lnot
%		\left(\begin{array}{l} \exists 	z_0 : S_{in\alpha P} \spot \\
%				 z_0 \in t \land (\bigwedge x : \alpha P \spot z_0.x = z.(x'))
%			\end{array}\right)
\end{flalign*}
\end{proof}
\end{law}

\begin{law}[$ac2acdash$-$\emptyset$]\label{law:ac2acdash:emptyset}
\begin{align*}
	&ac2acdash(\emptyset) = \emptyset&
\end{align*}
\begin{proof}
Similar to that of~\cref{law:acdash2ac:emptyset}
\end{proof}
\end{law}

\section{$\mathbf{PBMH}$}

\begin{law}\label{law:pmbh:P-empty-ac'-or-P} Provided $P$ satisfies $\mathbf{PBMH}$.
\begin{align*}
	&P[\emptyset/ac'] \lor P = P&
\end{align*}
\begin{proof}
\begin{flalign*}
	&P[\emptyset/ac'] \lor P
	&&\ptext{Assumption: $P$ is $\mathbf{PBMH}$-healthy}\\
	&=(P \circseq ac \subseteq ac')[\emptyset/ac'] \lor (P \circseq ac \subseteq ac')
	&&\ptext{Substitution}\\
	&=(P \circseq ac \subseteq \emptyset) \lor (P \circseq ac \subseteq ac')
	&&\ptext{Distributivity of sequential composition w.r.t. disjunction}\\
	&=P \circseq (ac \subseteq \emptyset \lor ac \subseteq ac')
	&&\ptext{Property of subset inclusion}\\
	&=P \circseq (ac \subseteq ac')
	&&\ptext{Assumption: $P$ is $\mathbf{PBMH}$-healthy}\\
	&=P
\end{flalign*}
\end{proof}
\end{law}

\section{Lemmas}

\begin{lemma}\label{lemma:pbmh2d:ac'-neq-empty}
\begin{align*}
	&pbmh2d(P) = \left(\begin{array}{l}
			\lnot P[\emptyset/ac'][s/in\alpha] 
			\\ \vdash \\
			\exists ac_0 \spot P[ac_0/ac'][s/in\alpha] \land acdash2ac(ac_0) \subseteq ac' \land ac'\neq\empty
		\end{array}\right)
\end{align*}
\begin{proof}
\begin{flalign*}
	&pbmh2d(P)
	&&\ptext{Definition of $pbmh2d$}\\
	&=\left(\begin{array}{l}
			\lnot P[\emptyset/ac'][s/in\alpha] 
			\\ \vdash \\
			\exists ac_0 \spot P[ac_0/ac'][s/in\alpha] \land acdash2ac(ac_0) \subseteq ac'
		\end{array}\right)
	&&\ptext{Predicate calculus}\\
	&=\left(\begin{array}{l}
			\lnot P[\emptyset/ac'][s/in\alpha] 
			\\ \vdash \\
			\exists ac_0 \spot P[ac_0/ac'][s/in\alpha] \land acdash2ac(ac_0) \subseteq ac' \\
			\land (ac'=\emptyset \lor ac'\neq\emptyset)
		\end{array}\right)
	&&\ptext{Predicate calculus}\\
	&=\left(\begin{array}{l}
			\lnot P[\emptyset/ac'][s/in\alpha] 
			\\ \vdash \\
			\left(\begin{array}{l}
				(\exists ac_0 \spot P[ac_0/ac'][s/in\alpha] \land acdash2ac(ac_0) \subseteq ac' \land ac'\neq\emptyset) 
				\\ \lor \\
				(\exists ac_0 \spot P[ac_0/ac'][s/in\alpha] \land acdash2ac(ac_0) \subseteq ac' \land ac'=\emptyset)
			\end{array}\right)
		\end{array}\right)
	&&\ptext{Property of sets}\\
	&=\left(\begin{array}{l}
			\lnot P[\emptyset/ac'][s/in\alpha] 
			\\ \vdash \\
			\left(\begin{array}{l}
				(\exists ac_0 \spot P[ac_0/ac'][s/in\alpha] \land acdash2ac(ac_0) \subseteq ac' \land ac'\neq\emptyset) 
				\\ \lor \\
				\left(\begin{array}{l}
					\exists ac_0 \spot P[ac_0/ac'][s/in\alpha] \land \\
					\forall z \spot (z \in acdash2ac(ac_0) \implies z \in ac') \land \forall z \spot z \notin ac'
				\end{array}\right)
			\end{array}\right)
		\end{array}\right)
	&&\ptext{Predicate calculus}\\
	&=\left(\begin{array}{l}
			\lnot P[\emptyset/ac'][s/in\alpha] 
			\\ \vdash \\
			\left(\begin{array}{l}
				(\exists ac_0 \spot P[ac_0/ac'][s/in\alpha] \land acdash2ac(ac_0) \subseteq ac' \land ac'\neq\emptyset) 
				\\ \lor \\
				\left(\begin{array}{l}
					\exists ac_0 \spot P[ac_0/ac'][s/in\alpha] \land \\
					\forall z \spot (z \notin acdash2ac(ac_0) \land z \notin ac')
				\end{array}\right)
			\end{array}\right)
		\end{array}\right)
	&&\ptext{Property of sets}\\
	&=\left(\begin{array}{l}
			\lnot P[\emptyset/ac'][s/in\alpha] 
			\\ \vdash \\
			\left(\begin{array}{l}
				(\exists ac_0 \spot P[ac_0/ac'][s/in\alpha] \land acdash2ac(ac_0) \subseteq ac' \land ac'\neq\emptyset) 
				\\ \lor \\
				\left(\begin{array}{l}
					\exists ac_0 \spot P[ac_0/ac'][s/in\alpha] \land
					\\ ac2acdash \circ acdash2ac(ac_0) = ac2acdash(\emptyset) \land ac'=\emptyset
				\end{array}\right)
			\end{array}\right)
		\end{array}\right)
	&&\ptext{\cref{law:ac2acdash:emptyset} and \cref{law:acdash2ac-ac2acdash}}\\
	&=\left(\begin{array}{l}
		\lnot P[\emptyset/ac'][s/in\alpha] 
		\\ \vdash \\
		\left(\begin{array}{l}
			(\exists ac_0 \spot P[ac_0/ac'][s/in\alpha] \land acdash2ac(ac_0) \subseteq ac' \land ac'\neq\emptyset) 
			\\ \lor \\
			(\exists ac_0 \spot P[ac_0/ac'][s/in\alpha] \land ac_0 = \emptyset \land ac'=\emptyset)
		\end{array}\right)
	\end{array}\right)
	&&\ptext{One-point rule}\\
	&=\left(\begin{array}{l}
		\lnot P[\emptyset/ac'][s/in\alpha] 
		\\ \vdash \\
		\left(\begin{array}{l}
			(\exists ac_0 \spot P[ac_0/ac'][s/in\alpha] \land acdash2ac(ac_0) \subseteq ac' \land ac'\neq\emptyset) 
			\\ \lor \\
			(P[\emptyset/ac'][s/in\alpha] \land ac'=\emptyset)
		\end{array}\right)
	\end{array}\right)
	&&\ptext{Definition of design}\\
	&=\left(\begin{array}{l}
		(ok \land \lnot P[\emptyset/ac'][s/in\alpha])
		\\ \implies \\
		\left(\begin{array}{l}
			(\exists ac_0 \spot P[ac_0/ac'][s/in\alpha] \land acdash2ac(ac_0) \subseteq ac' \land ac'\neq\emptyset \land ok') 
			\\ \lor \\
			(P[\emptyset/ac'][s/in\alpha] \land ac'=\emptyset \land ok')
		\end{array}\right)
	\end{array}\right)
	&&\ptext{Predicate calculus}\\
	&=\left(\begin{array}{l}
		ok \implies \\
		\left(\begin{array}{l}
			(\exists ac_0 \spot P[ac_0/ac'][s/in\alpha] \land acdash2ac(ac_0) \subseteq ac' \land ac'\neq\emptyset \land ok') 
			\\ \lor \\
			(P[\emptyset/ac'][s/in\alpha] \land ac'=\emptyset \land ok')
			\\ \lor \\
			P[\emptyset/ac'][s/in\alpha]
		\end{array}\right)
	\end{array}\right)
	&&\ptext{Predicate calculus: absorption law}\\
	&=\left(\begin{array}{l}
		ok \implies \\
		\left(\begin{array}{l}
			(\exists ac_0 \spot P[ac_0/ac'][s/in\alpha] \land acdash2ac(ac_0) \subseteq ac' \land ac'\neq\emptyset \land ok') 
			\\ \lor \\
			P[\emptyset/ac'][s/in\alpha]
		\end{array}\right)
	\end{array}\right)
	&&\ptext{Predicate calculus and definition of design}\\
	&=\left(\begin{array}{l}
		\lnot P[\emptyset/ac'][s/in\alpha]
		\\ \vdash \\
		\exists ac_0 \spot P[ac_0/ac'][s/in\alpha] \land acdash2ac(ac_0) \subseteq ac' \land ac'\neq\emptyset
	\end{array}\right)
\end{flalign*}
\end{proof}
\end{lemma}

\section{$d2pbmh$}

\begin{theorem}\label{theorem:d2pbmh:pbmh}
\begin{statement}Provided $P$ is $\mathbf{PBMH}$-healthy.
\begin{align*}
	&\mathbf{PBMH} \circ d2pbmh(P) = d2pbmh(P)
\end{align*}
\end{statement}
\begin{proofs}
\begin{proof}
\begin{xflalign*}
	&\mathbf{PBMH} \circ d2pbmh(P)
	&&\ptext{Assumption: $P$ is $\mathbf{PBMH}$-healthy and~\cref{lemma:d2pbmh-o-PBMH(P)}}\\
	&=\exists ac_0 @ \left(\begin{array}{l}
			(\lnot P^f \implies P^t)[true/ok][State_{\II}(in\alpha_{-ok})/s][ac_0/ac']
			\\ \land \\
			ac_0\subseteq undashset(ac')
	\end{array}\right)
	&&\ptext{Introduce fresh variable $ac_1$}\\
	&=\exists ac_0, ac_1 @ \left(\begin{array}{l}
			(\lnot P^f \implies P^t)[true/ok][State_{\II}(in\alpha_{-ok})/s][ac_0/ac']
			\\ \land \\
			ac_0\subseteq undashset(ac_1) \land	undashset(ac_1)\subseteq undashset(ac')
	\end{array}\right)
	&&\ptext{Property of $undashset$}\\
	&=\exists ac_0, ac_1 @ \left(\begin{array}{l}
			(\lnot P^f \implies P^t)[true/ok][State_{\II}(in\alpha_{-ok})/s][ac_0/ac']
			\\ \land \\
			ac_0\subseteq undashset(ac_1) \land	ac_1\subseteq ac'
	\end{array}\right)
	&&\ptext{Substitution and predicate calculus}\\
	&=\exists ac_1 @ \left(\exists ac_0 @ \left(\begin{array}{l}
			(\lnot P^f \implies P^t)[true/ok][State_{\II}(in\alpha_{-ok})/s][ac_0/ac']
			\\ \land \\
			ac_0\subseteq undashset(ac')\end{array}\right)[ac_1/ac'] \land	ac_1\subseteq ac'
	\right)
	&&\ptext{Definition of $\mathbf{PBMH}$}\\
	&=\left(\exists ac_0 @ \left(\begin{array}{l}
			(\lnot P^f \implies P^t)[true/ok][State_{\II}(in\alpha_{-ok})/s][ac_0/ac']
			\\ \land \\
			ac_0\subseteq undashset(ac')
	\end{array}\right)\right)
	&&\ptext{Assumption: $P$ is $\mathbf{PBMH}$-healthy and~\cref{lemma:d2pbmh-o-PBMH(P)}}\\
	&=d2pbmh(P)
\end{xflalign*}
\end{proof}
\end{proofs}
\end{theorem}\noindent

\begin{lemma}\label{lemma:d2pbmh-o-PBMH(P)}
\begin{statement}
\begin{align*}
	&d2pbmh \circ \mathbf{PBMH} (P)\\
	&=\\
	&\exists ac_0 @ \left(\begin{array}{l}
			(\lnot P^f \implies P^t)[true/ok][State_{\II}(in\alpha_{-ok})/s][ac_0/ac']
			\\ \land \\
			ac_0\subseteq undashset(ac')
	\end{array}\right)
\end{align*}
\end{statement}
\begin{proofs}
\begin{proof}
\begin{xflalign*}
	&d2pbmh \circ \mathbf{PBMH} (P)
	&&\ptext{Definition of $d2pbmh$}\\
	&=(\lnot \mathbf{PBMH} (P)^f \implies \mathbf{PBMH} (P)^t)[true/ok][undashset(ac')/ac'][State_{\II}(in\alpha_{-ok})/s]
	&&\ptext{\cref{lemma:PBMH(P)-ow:PBMH(P-ow)}}\\
	&=(\lnot \mathbf{PBMH} (P^f) \implies \mathbf{PBMH} (P^t))[true/ok][undashset(ac')/ac'][State_{\II}(in\alpha_{-ok})/s]
	&&\ptext{Predicate calculus and~\cref{law:pbmh:distribute-disjunction}}\\
	&=\mathbf{PBMH} (\lnot P^f \implies P^t)[true/ok][undashset(ac')/ac'][State_{\II}(in\alpha_{-ok})/s]
	&&\ptext{Definition of $\mathbf{PBMH}$}\\
	&=(\exists ac_0 @ (\lnot P^f \implies P^t)[ac_0/ac'] \land ac_0\subseteq ac')[true/ok][undashset(ac')/ac'][State_{\II}(in\alpha_{-ok})/s]
	&&\ptext{Substitution}\\
	&=\exists ac_0 @ \left(\begin{array}{l}
			(\lnot P^f \implies P^t)[true/ok][State_{\II}(in\alpha_{-ok})/s][ac_0/ac']
			\\ \land \\
			ac_0\subseteq undashset(ac')
	\end{array}\right)
\end{xflalign*}
\end{proof}
\end{proofs}
\end{lemma}

\begin{lemma}\label{lemma:PBMH(P)-subs-f-ac'}
\begin{statement}
Provided $f$ is bijective.
\begin{align*}
	&\mathbf{PBMH} (P)[f(ac')/ac'] = \mathbf{PBMH} (P[f(ac')/ac'])
\end{align*}
\end{statement}
\begin{proofs}
\begin{proof}
\begin{xflalign*}
	&\mathbf{PBMH} (P[f(ac')/ac'])
	&&\ptext{Definition of $\mathbf{PBMH}$}\\
	&=\exists ac_0 @ P[f(ac')/ac'][ac_0/ac'] \land ac_0\subseteq ac'
	&&\ptext{Substitution}\\
	&=\exists ac_0 @ P[f(ac_0)/ac'] \land ac_0\subseteq ac'
	&&\ptext{Predicate calculus}\\
	&=\exists ac_0 @ (\exists ac_1 @ P[ac_1/ac'] \land ac_1 = f(ac_0)) \land ac_0\subseteq ac'
	&&\ptext{Assumption: $f$ is bijective}\\
	&=\exists ac_0 @ (\exists ac_1 @ P[ac_1/ac'] \land f^{-1} (ac_1) = ac_0) \land ac_0\subseteq ac'
	&&\ptext{One-point rule}\\
	&=\exists ac_1 @ P[ac_1/ac'] \land f^{-1} (ac_1)\subseteq ac'
	&&\ptext{Assumption: $f$ is bijective}\\
	&=\exists ac_1 @ P[ac_1/ac'] \land ac_1\subseteq f(ac')
	&&\ptext{Substitution}\\
	&=(\exists ac_1 @ P[ac_1/ac'] \land ac_1\subseteq ac')[f(ac')/ac']
	&&\ptext{Definition of $\mathbf{PBMH}$}\\
	&=\mathbf{PBMH} (P)[f(ac')/ac']
\end{xflalign*}
\end{proof}
\end{proofs}
\end{lemma}

\begin{lemma}\label{lemma:P-land-ac'-neq-emptyset:P-ac'-subs-emptyset}
\begin{statement}
$P \land ac'=\emptyset = P[\emptyset/ac'] \land ac'=\emptyset$
\end{statement}
\begin{proofs}
\begin{proof}
\begin{xflalign*}
	&P \land ac'=\emptyset
	&&\ptext{Predicate calculus and fresh variable}\\
	&=\exists ac_0 @ P[ac_0/ac'] \land ac'=ac_0 \land ac'=\emptyset
	&&\ptext{Transitivity of equality}\\
	&=\exists ac_0 @ P[ac_0/ac'] \land ac'=\emptyset \land ac'=\emptyset
	&&\ptext{One-point rule}\\
	&=P[\emptyset/ac'] \land ac'=\emptyset
\end{xflalign*}
\end{proof}
\end{proofs}
\end{lemma}

\begin{theorem}\label{theorem:A-o-H3-o-pbmh2d(P):pbmh2d(P)}
\begin{statement}
Provided $P$ is $\mathbf{PBMH}$-healthy.
\begin{align*}
	&\mathbf{A} \circ \mathbf{H3} \circ pbmh2d(P) = pbmh2d(P)
\end{align*}
\end{statement}
\begin{proofs}
\begin{proof}
\begin{xflalign*}
	&\mathbf{A} \circ \mathbf{H3} \circ pbmh2d(P)
	&&\ptext{Definition of $pbmh2d$}\\
	&=\mathbf{A} \circ \mathbf{H3} ((\lnot P[\emptyset/ac'] \vdash P[dashset(ac')/ac'])[\mathbf{s}/in\alpha_{-ok}])
	&&\ptext{Substitution}\\
	&=\mathbf{A} \circ \mathbf{H3} ((\lnot P[\emptyset/ac'][\mathbf{s}/in\alpha_{-ok}] \vdash P[dashset(ac')/ac'][\mathbf{s}/in\alpha_{-ok}]))
	&&\ptext{Definition of $\mathbf{A}$ and $\mathbf{H3}$}\\
	&=\left(\begin{array}{l}
		\exists ac' @ \lnot P[\emptyset/ac'][\mathbf{s}/in\alpha_{-ok}]
		\\ \vdash \\
		\mathbf{PBMH} (P[dashset(ac')/ac'][\mathbf{s}/in\alpha_{-ok}]) \land ac'\neq\emptyset
	\end{array}\right)
	&&\ptext{$ac'$ not free}\\
	&=\left(\begin{array}{l}
		\lnot P[\emptyset/ac'][\mathbf{s}/in\alpha_{-ok}]
		\\ \vdash \\
		\mathbf{PBMH} (P[dashset(ac')/ac'][\mathbf{s}/in\alpha_{-ok}]) \land ac'\neq\emptyset
	\end{array}\right)
	&&\ptext{Substitution and definition of $\mathbf{PBMH}$}\\
	&=\left(\begin{array}{l}
		\lnot P[\emptyset/ac'][\mathbf{s}/in\alpha_{-ok}]
		\\ \vdash \\
		\mathbf{PBMH} (P[dashset(ac')/ac'])[\mathbf{s}/in\alpha_{-ok}] \land ac'\neq\emptyset
	\end{array}\right)
	&&\ptext{\cref{lemma:PBMH(P)-subs-f-ac'}}\\
	&=\left(\begin{array}{l}
		\lnot P[\emptyset/ac'][\mathbf{s}/in\alpha_{-ok}]
		\\ \vdash \\
		\mathbf{PBMH} (P)[dashset(ac')/ac'][\mathbf{s}/in\alpha_{-ok}] \land ac'\neq\emptyset
	\end{array}\right)
	&&\ptext{Assumption: $P$ is $\mathbf{PBMH}$-healthy}\\
	&=\left(\begin{array}{l}
		\lnot P[\emptyset/ac'][\mathbf{s}/in\alpha_{-ok}]
		\\ \vdash \\
		P[dashset(ac')/ac'][\mathbf{s}/in\alpha_{-ok}] \land ac'\neq\emptyset
	\end{array}\right)
	&&\ptext{Property of designs}\\
	&=\left(\begin{array}{l}
		\lnot P[\emptyset/ac'][\mathbf{s}/in\alpha_{-ok}]
		\\ \vdash \\
		(P[\emptyset/ac'][\mathbf{s}/in\alpha_{-ok}]) \lor (P[dashset(ac')/ac'][\mathbf{s}/in\alpha_{-ok}] \land ac'\neq\emptyset)
	\end{array}\right)
	&&\ptext{\cref{lemma:P-land-ac'-neq-emptyset:P-ac'-subs-emptyset}}\\
	&=\left(\begin{array}{l}
		\lnot P[\emptyset/ac'][\mathbf{s}/in\alpha_{-ok}]
		\\ \vdash \\
		(P[\mathbf{s}/in\alpha_{-ok}] \land ac'=\emptyset) \lor (P[dashset(ac')/ac'][\mathbf{s}/in\alpha_{-ok}] \land ac'\neq\emptyset)
	\end{array}\right)
	&&\ptext{Property of $dashset$}\\
	&=\left(\begin{array}{l}
		\lnot P[\emptyset/ac'][\mathbf{s}/in\alpha_{-ok}]
		\\ \vdash \\
		\left(\begin{array}{l}
			(P[dashset(ac')/ac'][\mathbf{s}/in\alpha_{-ok}] \land ac'=\emptyset)
			\\ \lor \\
			(P[dashset(ac')/ac'][\mathbf{s}/in\alpha_{-ok}] \land ac'\neq\emptyset)
		\end{array}\right)
	\end{array}\right)
	&&\ptext{Predicate calculus}\\
	&=\left(\begin{array}{l}
		\lnot P[\emptyset/ac'][\mathbf{s}/in\alpha_{-ok}]
		\\ \vdash \\
		P[dashset(ac')/ac'][\mathbf{s}/in\alpha_{-ok}] \land ac'=\emptyset
	\end{array}\right)
	&&\ptext{Definition of $pbmh2d$}\\
	&=pbmh2d(P)
\end{xflalign*}
\end{proof}
\end{proofs}
\end{theorem}

\begin{theorem}\label{theorem:d2pbm-o-pbmh2d(P):P}
\begin{statement}
Provided $P$ is $\mathbf{PBMH}$-healthy. $d2pbmh \circ pbmh2d(P) = P$
\end{statement}
\begin{proofs}
\begin{proof}
\begin{xflalign*}
	&d2pbmh \circ pbmh2d(P)
	&&\ptext{Definition of $d2pbmh$}\\
	&=(\lnot (pbmh2d(P))^f \implies (pbmh2d(P))^t)[true/ok][undashset(ac')/ac'][State_{\II}(in\alpha_{-ok})/s]
	&&\ptext{Definition of $pbmh2d$ and~\cref{lemma:design:(P|-Q)f:ok-implies-lnot-Pf,lemma:design(P|-Q)t:ok-land-Pt-implies-Qt}}\\
	&=\left(\begin{array}{l}
		\lnot (ok \implies P[\emptyset/ac'][\mathbf{s}/in\alpha_{-ok}]^f)
		\\ \implies \\
		\left(\begin{array}{l}
			(ok \land P[\emptyset/ac'][\mathbf{s}/in\alpha_{-ok}]^f)
			\\ \implies \\
			P[dashset(ac')/ac'][\mathbf{s}/in\alpha_{-ok}]^t)
		\end{array}\right)
	\end{array}\right)[true/ok][undashset(ac')/ac'][State_{\II}(in\alpha_{-ok})/s]
	&&\ptext{Substitution}\\
	&=\left(\begin{array}{l}
		\lnot P[\emptyset/ac'][\mathbf{s}/in\alpha_{-ok}]^f
		\\ \implies \\
		\left(\begin{array}{l}
			(P[\emptyset/ac'][\mathbf{s}/in\alpha_{-ok}]^f)
			\\ \implies \\
			P[dashset(ac')/ac'][\mathbf{s}/in\alpha_{-ok}]^t)
		\end{array}\right)
	\end{array}\right)[undashset(ac')/ac'][State_{\II}(in\alpha_{-ok})/s]
	&&\ptext{$ok'$ not free in $P$}\\
	&=\left(\begin{array}{l}
		\lnot P[\emptyset/ac'][\mathbf{s}/in\alpha_{-ok}]
		\\ \implies \\
		\left(\begin{array}{l}
			(P[\emptyset/ac'][\mathbf{s}/in\alpha_{-ok}])
			\\ \implies \\
			(P[dashset(ac')/ac'][\mathbf{s}/in\alpha_{-ok}])
		\end{array}\right)
	\end{array}\right)[undashset(ac')/ac'][State_{\II}(in\alpha_{-ok})/s]
	&&\ptext{Predicate calculus}\\
	&=\left(\begin{array}{l}
		\lnot P[\emptyset/ac'][\mathbf{s}/in\alpha_{-ok}]
		\\ \implies \\
		P[dashset(ac')/ac'][\mathbf{s}/in\alpha_{-ok}]
	\end{array}\right)[undashset(ac')/ac'][State_{\II}(in\alpha_{-ok})/s]
	&&\ptext{Substitution}\\
	&=\left(\begin{array}{l}
		\lnot P[\emptyset/ac'][\mathbf{s}/in\alpha_{-ok}][State_{\II}(in\alpha_{-ok})/s]
		\\ \implies \\
		P[dashset \circ undashset(ac')/ac'][\mathbf{s}/in\alpha_{-ok}][State_{\II}(in\alpha_{-ok})/s]
	\end{array}\right)
	&&\ptext{Property of $dashset$ and $undashset$}\\
	&=\left(\begin{array}{l}
		\lnot P[\emptyset/ac'][\mathbf{s}/in\alpha_{-ok}][State_{\II}(in\alpha_{-ok})/s]
		\\ \implies \\
		P[\mathbf{s}/in\alpha_{-ok}][State_{\II}(in\alpha_{-ok})/s]
	\end{array}\right)
	&&\ptext{\cref{lemma:state-sub:P-z-S:S-z}}\\
	&=(\lnot P[\emptyset/ac'] \implies P)
	&&\ptext{Predicate calculus}\\
	&=P[\emptyset/ac'] \lor P
	&&\ptext{Assumption: $P$ is $\mathbf{PBMH}$-healthy and~\cref{law:pmbh:P-empty-ac'-or-P}}\\
	&=P
\end{xflalign*}
\end{proof}
\end{proofs}
\end{theorem}

\begin{lemma}\label{lemma:pbmh2d-o-d2pbmh(P)}
\begin{statement}
\begin{align*}
	&pbmh2d \circ d2pbmh(P) = (\lnot P^f[\emptyset/ac'] \land \lnot P^t[\emptyset/ac'] \vdash (\lnot P^f \implies P^t))
\end{align*}
\end{statement}
\begin{proofs}
\begin{proof}
\begin{xflalign*}
	&pbmh2d \circ d2pbmh(P)
	&&\ptext{Definition of $pbmh2d$}\\
	&=(\lnot d2pbmh(P)[\emptyset/ac'] \vdash d2pbmh(P)[dashset(ac')/ac'])[\mathbf{s}/in\alpha_{-ok}]
	&&\ptext{Definition of $d2pbmh$}\\
	&=\left(\begin{array}{l}
		\lnot (\lnot P^f \implies P^t)[true/ok][undashset(ac')/ac'][State_{\II}(in\alpha_{-ok})/s][\emptyset/ac']
		\\ \vdash \\
		(\lnot P^f \implies P^t)[true/ok][undashset(ac')/ac'][State_{\II}(in\alpha_{-ok})/s][dashset(ac')/ac']
	\end{array}\right)[\mathbf{s}/in\alpha_{-ok}]
	&&\ptext{Substitution}\\
	&=\left(\begin{array}{l}
		\lnot (\lnot P^f \implies P^t)[true/ok][undashset(\emptyset)/ac'][State_{\II}(in\alpha_{-ok})/s]
		\\ \vdash \\
		(\lnot P^f \implies P^t)[true/ok][undashset \circ dashset(ac')/ac'][State_{\II}(in\alpha_{-ok})/s]
	\end{array}\right)[\mathbf{s}/in\alpha_{-ok}]
	&&\ptext{\cref{lemma:state-sub:P-S-z:z-S}}\\
	&=\left(\begin{array}{l}
		\lnot (\lnot P^f \implies P^t)[true/ok][undashset(\emptyset)/ac']
		\\ \vdash \\
		(\lnot P^f \implies P^t)[true/ok][undashset \circ dashset(ac')/ac']
	\end{array}\right)
	&&\ptext{$ok$ not free}\\
	&=\left(\begin{array}{l}
		\lnot (\lnot P^f \implies P^t)[undashset(\emptyset)/ac']
		\\ \vdash \\
		(\lnot P^f \implies P^t)[undashset \circ dashset(ac')/ac']
	\end{array}\right)
	&&\ptext{Property of $undashset$ and $dashset$}\\
	&=\left(\begin{array}{l}
		\lnot (\lnot P^f \implies P^t)[\emptyset/ac']
		\\ \vdash \\
		(\lnot P^f \implies P^t)
	\end{array}\right)
	&&\ptext{Substitution}\\
	&=(\lnot P^f[\emptyset/ac'] \land \lnot P^t[\emptyset/ac'] \vdash (\lnot P^f \implies P^t))
\end{xflalign*}
\end{proof}
\end{proofs}
\end{lemma}

\begin{theorem}\label{theorem:pbmh2d-o-d2pbmh(P):sqsubseteq:P}
\begin{statement}
Provided $P$ is an $\mathbf{A}$-healthy design.
\begin{align*}
	&pbmh2d \circ d2pbmh(P) \sqsubseteq P
\end{align*}
\end{statement}
\begin{proofs}
\begin{proof}
\begin{xflalign*}
	&pbmh2d \circ d2pbmh(P)
	&&\ptext{\cref{lemma:pbmh2d-o-d2pbmh(P)}}\\
	&=(\lnot P^f[\emptyset/ac'] \land \lnot P^t[\emptyset/ac'] \vdash (\lnot P^f \implies P^t))
	&&\ptext{Assumption: $P$ is an $\mathbf{A}$-healthy design}\\
	&=\left(\begin{array}{l}
			\left(\begin{array}{l}
				\lnot (\lnot \mathbf{PBMH} (P^f) \vdash \mathbf{PBMH} (P^t)\land ac'\neq\emptyset)^f[\emptyset/ac'] 
				\\ \land \\
				\lnot (\lnot \mathbf{PBMH} (P^f) \vdash \mathbf{PBMH} (P^t)\land ac'\neq\emptyset)^t[\emptyset/ac']
			\end{array}\right) 
			\\ \vdash \\
			\left(\begin{array}{l}
				\lnot (\lnot \mathbf{PBMH} (P^f) \vdash \mathbf{PBMH} (P^t)\land ac'\neq\emptyset)^f
				\\ \implies \\
				(\lnot \mathbf{PBMH} (P^f) \vdash \mathbf{PBMH} (P^t)\land ac'\neq\emptyset)^t
			\end{array}\right)
	\end{array}\right)
	&&\ptext{\cref{lemma:design(P|-Q)t:ok-land-Pt-implies-Qt,lemma:design:(P|-Q)f:ok-implies-lnot-Pf}}\\
	&=\left(\begin{array}{l}
			\left(\begin{array}{l}
				\lnot (ok \implies \mathbf{PBMH} (P^f)^f)[\emptyset/ac'] 
				\\ \land \\
				\lnot ((ok \land \lnot \mathbf{PBMH} (P^f)^t) \implies (\mathbf{PBMH} (P^t)\land ac'\neq\emptyset)^t)[\emptyset/ac']
			\end{array}\right) 
			\\ \vdash \\
			\left(\begin{array}{l}
				\lnot (ok \implies \mathbf{PBMH} (P^f)^f)
				\\ \implies \\
				((ok \land \lnot \mathbf{PBMH} (P^f)^t) \implies (\mathbf{PBMH} (P^t)\land ac'\neq\emptyset)^t)
			\end{array}\right)
	\end{array}\right)
	&&\ptext{$ok'$ not free}\\
	&=\left(\begin{array}{l}
			\left(\begin{array}{l}
				\lnot (ok \implies \mathbf{PBMH} (P^f))[\emptyset/ac'] 
				\\ \land \\
				\lnot ((ok \land \lnot \mathbf{PBMH} (P^f)) \implies (\mathbf{PBMH} (P^t)\land ac'\neq\emptyset))[\emptyset/ac']
			\end{array}\right) 
			\\ \vdash \\
			\left(\begin{array}{l}
				\lnot (ok \implies \mathbf{PBMH} (P^f))
				\\ \implies \\
				((ok \land \lnot \mathbf{PBMH} (P^f)) \implies (\mathbf{PBMH} (P^t)\land ac'\neq\emptyset))
			\end{array}\right)
	\end{array}\right)
	&&\ptext{Substitution}\\
	&=\left(\begin{array}{l}
			\left(\begin{array}{l}
				\lnot (ok \implies \mathbf{PBMH} (P^f)[\emptyset/ac']) 
				\\ \land \\
				\lnot ((ok \land \lnot \mathbf{PBMH} (P^f)) \implies (\mathbf{PBMH} (P^t)[\emptyset/ac']\land \emptyset\neq\emptyset))
			\end{array}\right) 
			\\ \vdash \\
			\left(\begin{array}{l}
				\lnot (ok \implies \mathbf{PBMH} (P^f))
				\\ \implies \\
				((ok \land \lnot \mathbf{PBMH} (P^f)) \implies (\mathbf{PBMH} (P^t)\land ac'\neq\emptyset))
			\end{array}\right)
	\end{array}\right)
	&&\ptext{Property of sets and predicate calculus}\\
	&=\left(\begin{array}{l}
			\left(\begin{array}{l}
				\lnot (ok \implies \mathbf{PBMH} (P^f)[\emptyset/ac']) 
				\\ \land \\
				(ok \land \lnot \mathbf{PBMH} (P^f))
			\end{array}\right) 
			\\ \vdash \\
			\left(\begin{array}{l}
				\lnot (ok \implies \mathbf{PBMH} (P^f))
				\\ \implies \\
				((ok \land \lnot \mathbf{PBMH} (P^f)) \implies (\mathbf{PBMH} (P^t)\land ac'\neq\emptyset))
			\end{array}\right)
	\end{array}\right)
	&&\ptext{Predicate calculus}\\
	&=\left(\begin{array}{l}
			\left(\begin{array}{l}
				(ok \land \lnot \mathbf{PBMH} (P^f)[\emptyset/ac']) 
				\\ \land \\
				(ok \land \lnot \mathbf{PBMH} (P^f))
			\end{array}\right) 
			\\ \vdash \\
			\left(\begin{array}{l}
				(ok \land \lnot \mathbf{PBMH} (P^f))
				\\ \implies \\
				((ok \land \lnot \mathbf{PBMH} (P^f)) \implies (\mathbf{PBMH} (P^t)\land ac'\neq\emptyset))
			\end{array}\right)
	\end{array}\right)
	&&\ptext{Property of designs and predicate calculus}\\
	&=\left(\begin{array}{l}
			\left(\begin{array}{l}
				(ok \land \lnot \mathbf{PBMH} (P^f)[\emptyset/ac']) 
				\\ \land \\
				(ok \land \lnot \mathbf{PBMH} (P^f))
			\end{array}\right) 
			\\ \vdash \\
			\mathbf{PBMH} (P^t) \land ac'\neq\emptyset
	\end{array}\right)
	&&\ptext{Property of designs and predicate calculus}\\
	&=\left(\begin{array}{l}
			\lnot \mathbf{PBMH} (P^f)[\emptyset/ac'] \land \lnot \mathbf{PBMH} (P^f)
			\\ \vdash \\
			\mathbf{PBMH} (P^t) \land ac'\neq\emptyset
	\end{array}\right)
	&&\ptext{Weaken precondition}\\
	&\sqsubseteq (\lnot \mathbf{PBMH} (P^f) \vdash \mathbf{PBMH} (P^t) \land ac'\neq\emptyset)
	&&\ptext{Definition of $\mathbf{A}$}\\
	&=\mathbf{A} (\lnot P^f \vdash P^t)
	&&\ptext{Assumption: $P$ is an~$\mathbf{A}$-healthy design}\\
	&=P
\end{xflalign*}
\end{proof}
\end{proofs}
\end{theorem}

\begin{theorem}\label{theorem:pbmh2d-o-d2pbmh(P):P}
\begin{statement}
Provided $P$ is design that is $\mathbf{A}$ and $\mathbf{H3}$-healthy.
\begin{align*}
	&pbmh2d \circ d2pbmh(P) = P
\end{align*}
\end{statement}
\begin{proofs}
\begin{proof}
\begin{xflalign*}
	&pbmh2d \circ d2pbmh(P)
	&&\ptext{\cref{lemma:pbmh2d-o-d2pbmh(P)}}\\
	&=(\lnot P^f[\emptyset/ac'] \land \lnot P^t[\emptyset/ac'] \vdash (\lnot P^f \implies P^t))
	&&\ptext{Assumption: $P$ is an design that is $\mathbf{A}$ and $\mathbf{H3}$-healthy}\\
	&=\left(\begin{array}{l}
			\left(\begin{array}{l}
				\lnot (\exists ac' @ \lnot P^f \vdash \mathbf{PBMH} (P^t)\land ac'\neq\emptyset)^f[\emptyset/ac'] 
				\\ \land \\
				\lnot (\exists ac' @ \lnot P^f \vdash \mathbf{PBMH} (P^t)\land ac'\neq\emptyset)^t[\emptyset/ac']
			\end{array}\right) 
			\\ \vdash \\
			\left(\begin{array}{l}
				\lnot (\exists ac' @ \lnot P^f \vdash \mathbf{PBMH} (P^t)\land ac'\neq\emptyset)^f
				\\ \implies \\
				(\exists ac' @ \lnot P^f \vdash \mathbf{PBMH} (P^t)\land ac'\neq\emptyset)^t
			\end{array}\right)
	\end{array}\right)
	&&\ptext{\cref{lemma:design(P|-Q)t:ok-land-Pt-implies-Qt,lemma:design:(P|-Q)f:ok-implies-lnot-Pf}}\\
	&=\left(\begin{array}{l}
			\left(\begin{array}{l}
				\lnot (ok \implies \lnot (\exists ac' @ \lnot P^f)^f)[\emptyset/ac'] 
				\\ \land \\
				\lnot ((ok \land (\exists ac' @ \lnot P^f)^t) \implies (\mathbf{PBMH} (P^t)\land ac'\neq\emptyset)^t)[\emptyset/ac']
			\end{array}\right) 
			\\ \vdash \\
			\left(\begin{array}{l}
				\lnot (ok \implies \lnot (\exists ac' @ \lnot P^f)^f)
				\\ \implies \\
				((ok \land (\exists ac' @ \lnot P^f)^t) \implies (\mathbf{PBMH} (P^t)\land ac'\neq\emptyset)^t)
			\end{array}\right)
	\end{array}\right)
	&&\ptext{$ok'$ not free}\\
	&=\left(\begin{array}{l}
			\left(\begin{array}{l}
				\lnot (ok \implies \lnot \exists ac' @ \lnot P^f)[\emptyset/ac'] 
				\\ \land \\
				\lnot ((ok \land (\exists ac' @ \lnot P^f)) \implies (\mathbf{PBMH} (P^t)\land ac'\neq\emptyset))[\emptyset/ac']
			\end{array}\right) 
			\\ \vdash \\
			\left(\begin{array}{l}
				\lnot (ok \implies \lnot (\exists ac' @ \lnot P^f))
				\\ \implies \\
				((ok \land (\exists ac' @ \lnot P^f)) \implies (\mathbf{PBMH} (P^t)\land ac'\neq\emptyset))
			\end{array}\right)
	\end{array}\right)
	&&\ptext{Substitution}\\
	&=\left(\begin{array}{l}
			\left(\begin{array}{l}
				\lnot (ok \implies \lnot \exists ac' @ \lnot P^f) 
				\\ \land \\
				\lnot ((ok \land \exists ac' @ \lnot P^f) \implies (\mathbf{PBMH} (P^t)[\emptyset/ac']\land \emptyset\neq\emptyset))
			\end{array}\right) 
			\\ \vdash \\
			\left(\begin{array}{l}
				\lnot (ok \implies \lnot (\exists ac' @ \lnot P^f))
				\\ \implies \\
				((ok \land \exists ac' @ \lnot P^f) \implies (\mathbf{PBMH} (P^t)\land ac'\neq\emptyset))
			\end{array}\right)
	\end{array}\right)
	&&\ptext{Property of sets and predicate calculus}\\
	&=\left(\begin{array}{l}
			\left(\begin{array}{l}
				\lnot (ok \implies \lnot \exists ac' @ \lnot P^f) 
				\\ \land \\
				(ok \land \exists ac' @ \lnot P^f)
			\end{array}\right) 
			\\ \vdash \\
			\left(\begin{array}{l}
				\lnot (ok \implies \lnot \exists ac' @ \lnot P^f)
				\\ \implies \\
				((ok \land \exists ac' @ \lnot P^f) \implies (\mathbf{PBMH} (P^t)\land ac'\neq\emptyset))
			\end{array}\right)
	\end{array}\right)
	&&\ptext{Predicate calculus}\\
	&=\left(\begin{array}{l}
			ok \land \exists ac' @ \lnot P^f
			\\ \vdash \\
			\left(\begin{array}{l}
				(ok \land \exists ac' @ \lnot P^f)
				\\ \implies \\
				((ok \land \exists ac' @ \lnot P^f) \implies (\mathbf{PBMH} (P^t)\land ac'\neq\emptyset))
			\end{array}\right)
	\end{array}\right)
	&&\ptext{Property of designs and predicate calculus}\\
	&=\left(\begin{array}{l}
			ok \land \exists ac' @ \lnot P^f 
			\\ \vdash \\
			\mathbf{PBMH} (P^t) \land ac'\neq\emptyset
	\end{array}\right)
	&&\ptext{Property of designs and predicate calculus}\\
	&=(\exists ac' @ \lnot P^f \vdash \mathbf{PBMH} (P^t) \land ac'\neq\emptyset)
	&&\ptext{Definition of $\mathbf{A}$ and $\mathbf{H3}$}\\
	&=\mathbf{A} \circ \mathbf{H3} (\lnot P^f \vdash P^t)
	&&\ptext{Assumption: $P$ is an design that is $\mathbf{A}$ and $\mathbf{H3}$-healthy}\\
	&=P
\end{xflalign*}
\end{proof}
\end{proofs}
\end{theorem}
