# Supplementary material for: Angelic Processes
Source: arXiv:1505.04726 source file (2015-05-28)
Supplement: Supplementary file 3 [file appendix-designs.tex]

\chapter{Theory of designs}
\label{appendix:designs:healthiness-conditions}

\section{Healthiness conditions}

\subsection*{$\mathbf{H2A}$}

\begin{define}
\begin{align*}
	&\mathbf{H2A} (P) \circdef \lnot P^f \implies (P^t \land ok')
\end{align*}
\end{define}

\begin{law}[$\mathbf{H2A} \iff \mathbf{H2}$]
The definition of $\mathbf{H2A}$ implies that the fixpoints are the same as those of $\mathbf{H2}$.
\begin{proof}[Proof for implication] The following proof is based on~\cite{Woodcock1996}.
\begin{flalign*}
	&P
	&&\ptext{Introduce fresh variable and substitution}\\
	&= \exists ok_0 \spot P \land ok'=ok_0
	&&\ptext{Case-split on $ok_0$}\\
	&= (\lnot ok' \land P^f) \lor (ok' \land P^t)
	&&\ptext{Assumption: P is $\mathbf{H2}$-healthy}\\
	&= (\lnot ok' \land P^f \land P^t) \lor (ok' \land P^t)
	&&\ptext{Propositional calculus}\\
	&= (((\lnot ok' \land P^f) \lor ok') \land P^t)
	&&\ptext{Propositional calculus}\\
	&= ((P^f \lor ok') \land P^t)
	&&\ptext{Propositional calculus}\\
	&= (P^f \land P^t) \lor (ok' \land P^t)
	&&\ptext{Assumption: P is $\mathbf{H2}$-healthy}&\\
	&= P^f \lor (ok' \land P^t)
	&&\ptext{Propositional calculus}\\
	&= \lnot P^f \implies (P^t \land ok')
\end{flalign*}
\end{proof}
\begin{proof}[Proof for reverse implication]
\begin{flalign*}
	&[(\mathbf{H2A} (P))^f \implies (\mathbf{H2A} (P))^t]
	&&\ptext{Definition of $\mathbf{H2A}$}\\
	&=[(\lnot P^f \implies (P^t \land ok'))^f \implies (\lnot P^f \implies (P^t \land ok'))^t]
	&&\ptext{Substitution}\\
	&=[(P^f \implies (\lnot P^f \implies P^t)]
	&&\ptext{Propositional calculus}\\
	&=[\lnot P^f \lor P^f \lor P^t]
	&&\ptext{Propositional calculus}\\
	&=true
\end{flalign*}
\end{proof}
\end{law}

\section{Lemmas}

\begin{lemma}[design-true-$ok'$]\label{law:design:true-ok'}
Provided $ok \land P$ and $ok'$ is not free in $P$.
\begin{align*}
	&(P \vdash Q)^t = Q
\end{align*}
\begin{proof}As stated and proved in~\cite{Cavalcanti2011a} (Lemma 4.2).\end{proof}
\end{lemma}

\begin{lemma}[design-false-$ok'$]\label{law:design:false-ok'}
Provided $ok'$ is not free in $P$.
\begin{align*}
	&ok \land \lnot(P \vdash Q)^f = ok \land P
\end{align*}
\begin{proof}As stated and proved in~\cite{Cavalcanti2011a} (Lemma 4.3).\end{proof}
\end{lemma}

\begin{lemma}[design-exists-$ok'$]\label{law:design:exists-ok'}
\begin{align*}
	&\exists ok' \spot (P \vdash Q) = (ok \land P) \implies Q
\end{align*}
\begin{proof}
\begin{flalign*}
	&\exists ok' \spot (P \vdash Q)
	&&\ptext{Definition of design}\\
	&=\exists ok' \spot (ok \land P) \implies (Q \land ok')
	&&\ptext{Case-split on $ok'$}\\
	&=((ok \land P) \implies Q) \lor \lnot (ok \land P)
	&&\ptext{Propositional calculus}\\
	&=(ok \land P) \implies Q
\end{flalign*}
\end{proof}
\end{lemma}

\begin{lemma}[design-$\sqcup$]\label{law:design:sqcup}
\begin{align*}
	&(\lnot P^f \vdash P^t) \sqcup (\lnot Q^f \vdash Q^t) \\
	&=\\
	&(\lnot P^f \lor \lnot Q^f \vdash (\lnot P^f \implies P^t) \land (\lnot Q^f \implies Q^t))
\end{align*}
\begin{proof}
\begin{flalign*}
	&(\lnot P^f \vdash P^t) \sqcup (\lnot Q^f \vdash Q^t)
	&&\ptext{Definition of design}\\
	&=((ok \land \lnot P^f) \implies (P^t \land ok')) \sqcup ((ok \land \lnot Q^f) \implies (Q^t \land ok'))
	&&\ptext{Definition of $\sqcup$}\\
	&=((ok \land \lnot P^f) \implies (P^t \land ok')) \land ((ok \land \lnot Q^f) \implies (Q^t \land ok'))
	&&\ptext{Propositional calculus}\\
	&=ok \implies ((P^t \land ok') \lor P^f) \land ((Q^t \land ok') \lor Q^f)
	&&\ptext{Propositional calculus}\\
	&=ok \implies (P^t \lor P^f) \land (ok' \lor P^f) \land (Q^t \lor Q^f) \land (ok' \lor Q^f)
	&&\ptext{Propositional calculus}\\
	&=ok \implies (P^t \lor P^f) \land (Q^t \lor Q^f) \land (ok' \lor (P^f \land Q^f))
	&&\ptext{Propositional calculus: absorption law}\\
	&=ok \implies ((P^f \land Q^f) \lor P^t \lor P^f) \land ((P^f \land Q^f) \lor Q^t \lor Q^f) \land (ok' \lor (P^f \land Q^f))
	&&\ptext{Propositional calculus}\\
	&=ok \implies (P^f \land Q^f) \lor ((P^t \lor P^f) \land (Q^t \lor Q^f) \land ok')
	&&\ptext{Propositional calculus}\\
	&=(ok \land \lnot (P^f \land Q^f)) \implies ((\lnot P^f \implies P^t) \land (\lnot Q^f \implies Q^t) \land ok')
	&&\ptext{Definition of design}\\
	&=(\lnot P^f \lor \lnot Q^f \vdash (\lnot P^f \implies P^t) \land (\lnot Q^f \implies Q^t))
\end{flalign*}
\end{proof}
\end{lemma}

\begin{lemma}[design-exists-ok'-$\sqcup$]\label{law:design:exists-ok':sqcup}
Provided $P$ and $Q$ are designs.
\begin{align*}
	&\exists ok' \spot (P \land Q) = (\exists ok' \spot P) \land (\exists ok' \spot Q)
\end{align*}
\begin{proof}
\begin{flalign*}
	&(\exists ok' \spot P) \land (\exists ok' \spot Q)
	&&\ptext{Assumption: $P$ and $Q$ are designs}\\
	&=(\exists ok' \spot (\lnot P^f \vdash P^t)) \land (\exists ok' \spot (\lnot Q^f \vdash Q^t))
	&&\ptext{\cref{law:design:exists-ok'}}\\
	&=((ok \land \lnot P^f ) \implies P^t) \land ((ok \land \lnot Q^f) \implies Q^t)
	&&\ptext{Propositional calculus}\\
	&=(ok \implies (P^t \lor P^f)) \land (ok \implies (Q^t \lor Q^f))
	&&\ptext{Propositional calculus}\\
	&=ok \implies ((P^t \lor P^f) \land (Q^t \lor Q^f))
	&&\ptext{Propositional calculus: absorption law}\\
	&=ok \implies (((P^f \land Q^f) \lor P^t \lor P^f) \land ((P^f \land Q^f) \lor Q^t \lor Q^f))
	&&\ptext{Propositional calculus}\\
	&=ok \implies ((P^f \land Q^f) \lor ((P^t \lor P^f) \land (Q^t \lor Q^f)))
	&&\ptext{Propositional calculus}\\
	&=(ok \land \lnot (P^f \land Q^f)) \implies ((\lnot P^f \implies P^t) \land (\lnot Q^f \implies Q^t))
	&&\ptext{\cref{law:design:exists-ok'}}\\
%	&=\exists ok' \spot (ok \land \lnot (P^f \land Q^f)) \implies ((\lnot P^f \implies P^t) \land (\lnot Q^f \implies Q^t) \land ok')
%	&&\ptext{Definition of design}\\
	&=\exists ok' \spot (\lnot (P^f \land Q^f) \vdash (\lnot P^f \implies P^t) \land (\lnot Q^f \implies Q^t))
	&&\ptext{Conjunction of designs}\\
	&=\exists ok' \spot (\lnot P^f \vdash P^t) \land (\lnot Q^f \vdash Q^t)
	&&\ptext{Assumption: $P$ and $Q$ are designs}\\
	&=\exists ok' \spot (P \land Q)
\end{flalign*}
\end{proof}
\end{lemma}

\begin{lemma}\label{law:designs:conjunction-alternative}
\begin{align*}
	&(\lnot P^f \vdash P^t) \sqcup (\lnot Q^f \vdash Q^t)\\
	&=\\
	&(\lnot P^f \lor \lnot Q^f \vdash (P^f \land Q^t) \lor (P^t \land Q^f) \lor (P^t \land Q^t))
\end{align*}
\begin{proof}
\begin{flalign*}
	&(\lnot P^f \vdash P^t) \sqcup (\lnot Q^f \vdash Q^t)
	&&\ptext{Conjunction of designs}\\
	&=(\lnot P^f \lor \lnot Q^f \vdash (\lnot P^f \implies P^t) \land (\lnot Q^f \implies Q^t))
	&&\ptext{Propositional calculus}\\
	&=(\lnot P^f \lor \lnot Q^f \vdash (P^f \lor P^t) \land (Q^f \lor Q^t))
	&&\ptext{Predicate calculus}\\
	&=(\lnot (P^f \land Q^f) \vdash (P^f \land Q^f) \lor (P^f \land Q^t) \lor (P^t \land Q^f) \lor (P^t \land Q^t))
	&&\ptext{Definition of design}\\
	&=\left(\begin{array}{l}
		(ok \land \lnot (P^f \land Q^f)) 
		\\ \implies \\
		(((P^f \land Q^f) \lor (P^f \land Q^t) \lor (P^t \land Q^f) \lor (P^t \land Q^t)) \land ok')
	\end{array}\right)
	&&\ptext{Predicate calculus}\\
	&=\left(\begin{array}{l}
		(ok \land \lnot (P^f \land Q^f) \land (\lnot (P^f \land Q^f) \lor \lnot ok')) 
		\\ \implies \\
		(((P^f \land Q^t) \lor (P^t \land Q^f) \lor (P^t \land Q^t)) \land ok')
	\end{array}\right)
	&&\ptext{Predicate calculus: absorption law}\\
	&=(ok \land \lnot (P^f \land Q^f)) \implies (((P^f \land Q^t) \lor (P^t \land Q^f) \lor (P^t \land Q^t)) \land ok')
	&&\ptext{Definition of design}\\
	&=(\lnot (P^f \land Q^f) \vdash (P^f \land Q^t) \lor (P^t \land Q^f) \lor (P^t \land Q^t))
	&&\ptext{Predicate calculus}\\
	&=(\lnot P^f \lor \lnot Q^f \vdash (P^f \land Q^t) \lor (P^t \land Q^f) \lor (P^t \land Q^t))
\end{flalign*}
\end{proof}
\end{lemma}

\begin{lemma}\label{lemma:design:(P|-Q)f:ok-implies-lnot-Pf}
\begin{align*}
	&(P \vdash Q)^f = ok \implies \lnot P^f
\end{align*}
\begin{proof}
\begin{xflalign*}
	&(P \vdash Q)^f
	&&\ptext{Definition of design}\\
	&=((ok \land P) \implies (Q \land ok'))^f
	&&\ptext{Substitution}\\
	&=((ok \land P^f) \implies (Q^f \land false))
	&&\ptext{Predicate calculus}\\
	&=\lnot (ok \land P^f)
	&&\ptext{Predicate calculus}\\
	&=ok \implies \lnot P^f
\end{xflalign*}
\end{proof}
\end{lemma}

\begin{lemma}\label{lemma:design(P|-Q)t:ok-land-Pt-implies-Qt}
\begin{align*}
	&(P \vdash Q)^t = (ok \land P^t) \implies Q^t
\end{align*}
\begin{proof}
\begin{xflalign*}
	&(P \vdash Q)^t
	&&\ptext{Definition of design}\\
	&=((ok \land P) \implies (Q \land ok'))^t
	&&\ptext{Substitution}\\
	&=((ok \land P^t) \implies (Q^t \land true))
	&&\ptext{Predicate calculus}\\
	&=(ok \land P^t) \implies Q^t
\end{xflalign*}
\end{proof}
\end{lemma}

\begin{lemma}\label{lemma:design:ok-land-lnot-exists(P|-Q)f:ok-land-lnot-exists-Pf}
\begin{align*}
	&ok \land \lnot \exists ac' \spot (P \vdash Q)^f = ok \land \lnot \exists ac' \spot \lnot P^f
\end{align*}
\begin{proof}
\begin{xflalign*}
	&ok \land \lnot \exists ac' \spot (P \vdash Q)^f
	&&\ptext{\cref{lemma:design:(P|-Q)f:ok-implies-lnot-Pf}}\\
	&=ok \land \lnot \exists ac' \spot (ok \implies \lnot P^f)
	&&\ptext{Predicate calculus}\\
	&=\lnot (\lnot ok \lor \exists ac' \spot (ok \implies \lnot P^f))
	&&\ptext{Predicate calculus}\\
	&=\lnot \exists ac' \spot (\lnot ok \lor (ok \implies \lnot P^f))
	&&\ptext{Predicate calculus}\\
	&=\lnot \exists ac' \spot (\lnot ok \lor \lnot P^f)
	&&\ptext{Predicate calculus}\\
	&=\lnot (\lnot ok \lor \exists ac' \spot \lnot P^f)
	&&\ptext{Predicate calculus}\\
	&=(ok \lor \lnot \exists ac' \spot \lnot P^f)
	&&\ptext{Predicate calculus}\\
	&=ok \land \lnot \exists ac' \spot \lnot P^f
\end{xflalign*}
\end{proof}
\end{lemma}

\begin{lemma}\label{lemma:design:(P|-Q)f-|-(P|-Q)t} Provided $ok$ is not free in $P$ and $Q$.
\begin{align*}
	&((P \vdash Q)^f \vdash (P \vdash Q)^t) = (P \vdash Q)
\end{align*}
\begin{proof}
\begin{xflalign*}
	&((P \vdash Q)^f \vdash (P \vdash Q)^t)
	&&\ptext{\cref{law:design:false-ok'}}\\
	&=(P \vdash (P \vdash Q)^t)
	&&\ptext{\cref{law:design:true-ok'}}\\
	&=(P \vdash Q)
\end{xflalign*}
\end{proof}
\end{lemma}

\begin{lemma}\label{lemma:design:(lnot-exists-ac'-(P|-Q)f-|-(P|-Q)t)} Provided $ok'$ is not free in $P$ and $Q$.
\begin{align*}
	&(\lnot \exists ac' \spot (P \vdash Q)^f \vdash (P \vdash Q)^t) = (\lnot \exists ac' \spot \lnot P \vdash Q)
\end{align*}
\begin{proof}
\begin{xflalign*}
	&(\lnot \exists ac' \spot (P \vdash Q)^f \vdash (P \vdash Q)^t)
	&&\ptext{Definition of design and~\cref{lemma:design:ok-land-lnot-exists(P|-Q)f:ok-land-lnot-exists-Pf}}\\
	&=(\lnot \exists ac' \spot \lnot P^f \vdash (P \vdash Q)^t)
	&&\ptext{Assumption: $ok'$ is not free in $P$}\\
	&=(\lnot \exists ac' \spot \lnot P \vdash (P \vdash Q)^t)
	&&\ptext{\cref{lemma:design(P|-Q)t:ok-land-Pt-implies-Qt}}\\
	&=(\lnot \exists ac' \spot \lnot P \vdash (ok \land P^t) \implies Q^t)
	&&\ptext{Assumption: $ok'$ not free in $P$ and $Q$}\\
	&=(\lnot \exists ac' \spot \lnot P \vdash (ok \land P) \implies Q)
	&&\ptext{Definition of design and predicate calculus}\\
	&=(\lnot \exists ac' \spot \lnot P \vdash P \implies Q)
	&&\ptext{Predicate calculus}\\
	&=(\lnot \exists ac' \spot \lnot P \vdash (\lnot P \land (\exists ac' \spot \lnot P)) \lor Q)
	&&\ptext{Definition of design and predicate calculus}\\
	&=(\lnot \exists ac' \spot \lnot P \vdash Q)
\end{xflalign*}
\end{proof}
\end{lemma}

\begin{lemma}\label{lemma:design:(lnot-(P|-Q)ff|-(P|-Q)tf)}
\begin{statement}
Provided $ok'$ is not free in $P$ and $Q$,
\begin{align*}
	&(\lnot (P \vdash Q)^f_f \vdash (P \vdash Q)^t_f) = (P_f \vdash Q_f)
\end{align*}
\end{statement}
\begin{proofs}
\begin{proof}
\begin{xflalign*}
	&(\lnot (P \vdash Q)^f_f \vdash (P \vdash Q)^t_f)
	&&\ptext{Definition of design}\\
	&=(\lnot ((ok \land P) \implies (Q \land ok'))^f_f \vdash ((ok \land P) \implies (Q \land ok'))^t_f)
	&&\ptext{Substitution}\\
	&=(\lnot ((ok \land P_f) \implies (Q_f \land false)) \vdash ((ok \land P_f) \implies (Q_f \land true)))
	&&\ptext{Predicate calculus}\\
	&=(ok \land P_f \vdash ((ok \land P_f) \implies Q_f))
	&&\ptext{Definition of design}\\
	&=(P_f \vdash ((ok \land P_f) \implies Q_f))
	&&\ptext{Definition of design and predicate calculus}\\
	&=(P_f \vdash Q_f)
\end{xflalign*}
\end{proof}
\end{proofs}
\end{lemma}

\subsection*{$\mathbf{H1}$}

\begin{lemma}\label{lemma:H1(P-cond-Q):H1(P)-cond-H1(Q)}
\begin{align*}
	&\mathbf{H1} (P \dres c \rres Q) = \mathbf{H1} (P) \dres c \rres \mathbf{H1} (Q)
\end{align*}
\begin{proof}\checkt{alcc}
\begin{xflalign*}
	&\mathbf{H1} (P) \dres c \rres \mathbf{H1} (Q)
	&&\ptext{Definition of $\mathbf{H1}$}\\
	&=(\lnot ok \lor P) \dres c \rres (\lnot ok \lor Q)
	&&\ptext{Property of conditional}\\
	&=(\lnot ok \dres c \rres \lnot ok) \lor (P \dres s.wait \rres Q)
	&&\ptext{Property of conditional}\\
	&=\lnot ok \lor (P \dres s.wait \rres Q)
	&&\ptext{Definition of $\mathbf{H1}$}\\
	&=\mathbf{H1} (P \dres s.wait \rres Q)
\end{xflalign*}
\end{proof}
\end{lemma}

\begin{lemma}\label{lemma:H1(P-land-Q):H1(P)-land-H1(Q)}
\begin{align*}
	&\mathbf{H1} (P \land Q) = \mathbf{H1} (P) \land \mathbf{H1} (Q)
\end{align*}
\begin{proof}
\begin{xflalign*}
	&\mathbf{H1} (P \land Q)
	&&\ptext{Definition of $\mathbf{H1}$}\\
	&=ok \implies (P \land Q)
	&&\ptext{Predicate calculus}\\
	&=(ok \implies P) \land (ok \implies Q)
	&&\ptext{Definition of $\mathbf{H1}$}\\
	&=\mathbf{H1} (P) \land \mathbf{H1} (Q)
\end{xflalign*}
\end{proof}
\end{lemma}

\begin{lemma}\label{lemma:H1(P-lor-Q):H1(P)-lor-H1(Q)}
\begin{align*}
	&\mathbf{H1} (P \lor Q) = \mathbf{H1} (P) \lor \mathbf{H1} (Q)
\end{align*}
\begin{proof}
\begin{xflalign*}
	&\mathbf{H1} (P \lor Q)
	&&\ptext{Definition of $\mathbf{H1}$}\\
	&=ok \implies (P \lor Q)
	&&\ptext{Predicate calculus}\\
	&=(ok \implies P) \lor (ok \implies Q)
	&&\ptext{Definition of $\mathbf{H1}$}\\
	&=\mathbf{H1} (P) \lor \mathbf{H1} (Q)
\end{xflalign*}
\end{proof}
\end{lemma}
